# Supplementary material for: Reverse epitaxy of Ge: ordered and facetted surface patterns
Source: arXiv:1303.5133 ancillary file (2013-03-21)
Supplement: Supplementary file 1 [file ReverseEpitaxySupplementalMaterial.pdf]

Supplemental Material for

"Reverse epitaxy of Ge: ordered and facetted surface patterns"

by Xin Ou, Adrian Keller, Manfred Helm, Jürgen Fassbender, and Stefan Facsko

### Numerical integration of the continuum equation

For the numerical integration of the continuum equation (Eqn. 1) we used a 4th order Runge-Kutta differentiation scheme with $\Delta x = \Delta y = 1$ and $\Delta t = 0.01$. For the nonlinear term $\nabla^2(\nabla h)^2$ we used the improved Lam-Shin discretization. We started the integration at t=0 with a flat surface $h(x, y)$ superimposed with white noise of amplitude of 0.1. As discussed in the paper the constant erosion rate, the curvature dependent sputtering, and mass redistribution by ion impact are negligible. Eqn. 1 is thus reduced to:

$$\frac{\partial h}{\partial t} = -\kappa \nabla^4 h - \sigma \nabla^2 (\nabla h)^2 - \epsilon \nabla \begin{bmatrix} m_x(1 - \delta m_x^2) \\ m_y(1 - \delta m_y^2) \end{bmatrix} . \quad (3)$$

The temporal evolution of the rms roughness and the characteristic length of the numerical integration with $\kappa = 4, \sigma = -1, \epsilon = 1$, and $\delta = 25$ are shown in Fig. S1. In the linear regime the surface roughness increases exponentially and the characteristic length is constant. Above 1000 s integration time the surface evolution enters the nonlinear regime where coarsening start. A roughening exponent of 0.45 and a coarsening exponent of 0.2 can be fitted to the data in the nonlinear regime in good agreement to the expected values of 1/2 and 1/4, respectively.

### Continuum equation at different temperatures

In our experiments we can identify four different temperature regimes for the pattern formation (see Fig. 1 in the paper). The proposed continuum equation (Eqn. 1) can describe all these regimes by choosing the proper coefficients. In Fig. S2 computed surfaces are shown for the different temperature regimes: (a) for T< 250°C (recrystallization temp of Ge), smoothing by ion irradiation and Herring Mullins diffusion dominates. In this case $\kappa = 1$, $\epsilon = -1$, $\sigma = -1$, and $\delta = 0$ in the continuum equation and the surface is smoothed. (b) For 250°C < T< 420°C checkerboard patterns are formed. In this regime the anisotropic

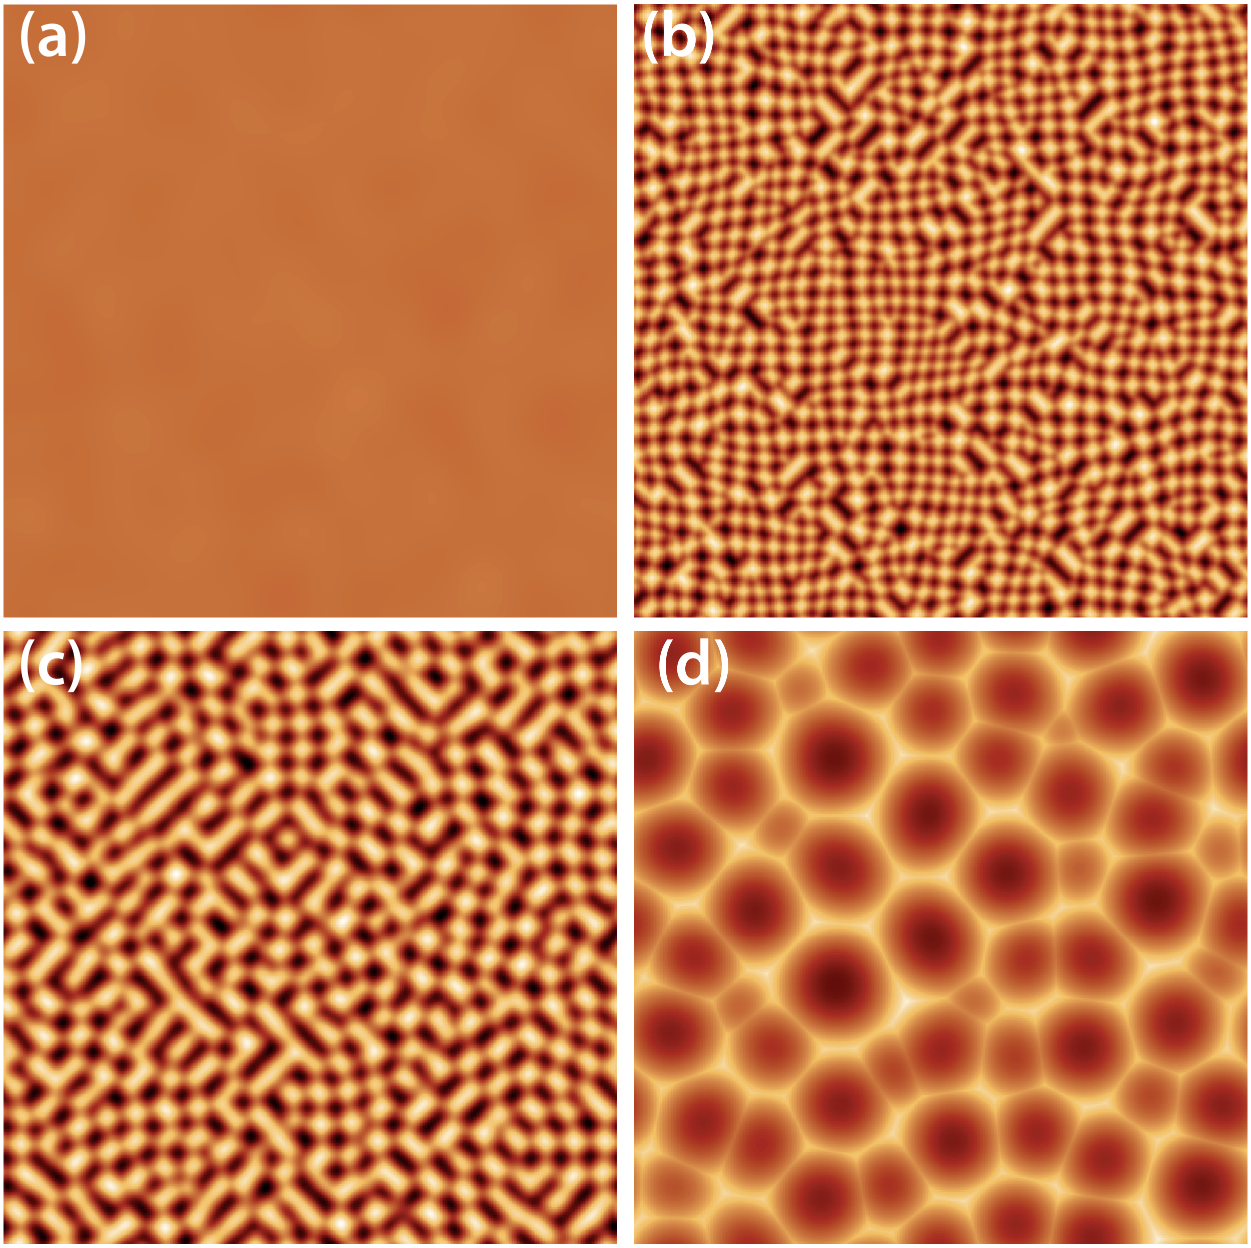


FIG. S1. Roughness, w, and characteristic length, $\lambda$, of surface patterns calculated by the continuum equation with the following parameters: $\kappa = 4, \sigma = -1, \epsilon = 1, \delta = 25$ on an integration grid of $400 \times 400$ points with $\Delta x = \Delta y = 1$, and $\Delta t = 0.01$.

ES barrier leads to a biased diffusion, $\epsilon = 1$, with anisotropic surface uphill current, $\delta \neq 0$, and thus to a surface instability. (c) The isotropic diffusion increases with temperature, thus $\kappa$ increases exponentially with temperature leading to an increase in the characteristic length of the checkerboard pattern. In Fig. S2c a surface diffusion coefficient $\kappa = 4$ was used. (d) For 420°C < T < 500°C we observe the transition from checkerboard to isotropic

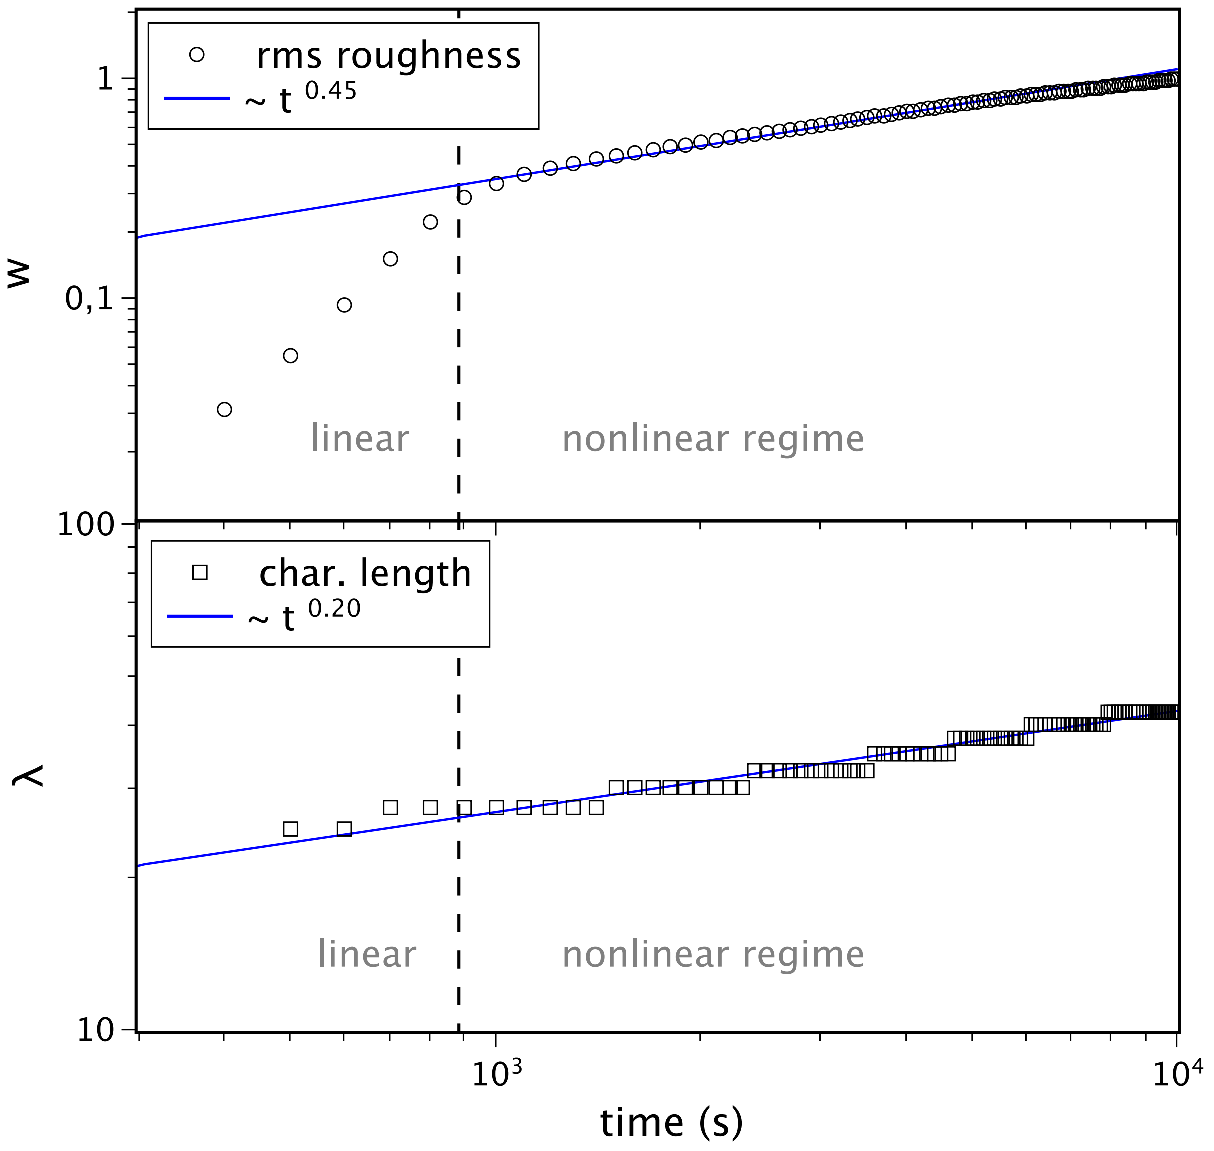


FIG. S2. Surface patterns computed by the continuum equation with different parameters: (a) $\kappa = 1, \sigma = -1, \epsilon = -1$, and $\delta = 0$, (b) $\kappa = 1, \sigma = -1, \epsilon = 1, \delta = 25$, (c) $\kappa = 4, \sigma = -1, \epsilon = 1, \delta = 25$, and (d) $\kappa = 4, \sigma = -1, \epsilon = 1, \delta = 0$ on an integration grid of $400 \times 400$ points with $\Delta x = \Delta y = 1$, and $\Delta t = 0.01$.

pit patterns. In this regime the ES barrier is still active, $\epsilon = 1$, however, isotropic and therefore $\delta = 0$. In this case the conserved KPZ term dominates and leads to isotropic patterns which coarsen with ion fluence. Finally, at T $>$ 500°C, the ES barrier is too weak to lead to an effective uphill current and smoothing dominates again, i.e. $\epsilon = -1$ (like in the low temperature regime).

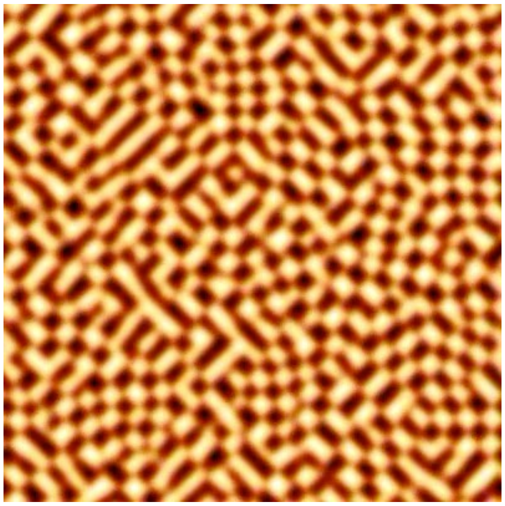

Video 1. Movie of the computed dynamical evolution of anisotropic, checkerboard patterns with the following parameters: $\kappa = 4, \sigma = -1, \epsilon = 1, \delta = 25$ (same as in Fig. S2c) corresponding to the regime with anisotropic terrace ES barrier.

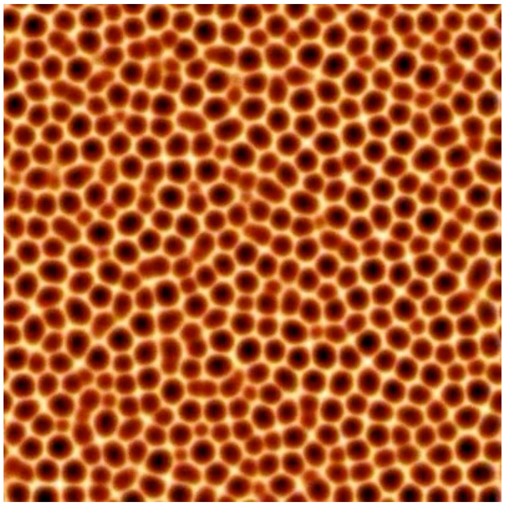

Video 2. Movie of the computed dynamical evolution of pit patterns in a "high temperature regime" with the following parameters: $\kappa = 4, \sigma = -1, \epsilon = 1, \delta = 0$ (same as in Fig. S2d) corresponding to the intermediate temperature regime with isotropic terrace ES barrier.

**Movies**

The temporal evolution of the surface height described by the continuum equation for the checkerboard pattern (Fig. S2c) and the isotropic pattern (Fig. S2d) can be seen in the following movies:
